# Supplementary material for: Boosting Visual Recognition in Real-world Degradations via Unsupervised Feature Enhancement Module with Deep Channel Prior
Source: arXiv:2404.01703 source file (2024-05-12)
Supplement: Supplementary file 1 [file X_suppl.tex]

\clearpage
\appendix
\setcounter{page}{1}
\maketitlesupplementary

\textbf{Overview:} In Section \ref{sec:sup_ablation}, we first emphasize the ablation study of our UFEM on real datasets to demonstrate its efficiency in real-world degradations. Then, we provide the Deep Channel Prior (DCP) in pre-trained ResNet50 to substantiate the universality and significance of our findings in Section \ref{sec:sup_dcp}. Besides, in Section \ref{sec:sup_config}, we present more empirical configurations within our method, \emph{e.g.}, the empirical weight values for each loss function and the structures of generator modules. In Section \ref{sec:sup_impl}, we further detail the implementation details in our experiments, including the eight benchmark datasets and the settings for each comparison method. Finally, more quantitative and qualitative analyses across three high-level vision tasks are displayed in Section \ref{sec:sup_exp}, such as results on Motion Blur and Low Contrast, Grad-CAM visualization comparison on other scenes, and so on. All the above validations further affirm the superiority of our proposed UFEM in various degradations, showcasing its universality across diverse tasks and datasets.

\section{Ablation Study on Real Datasets}
\label{sec:sup_ablation}

\section{Deep Channel Prior in ResNet50}
\label{sec:sup_dcp}
In the deep representation space, we can observe that highly sparse features with content loss and additional artifacts share a mixed and indistinguishable cluster. However, the correlations between feature channels exhibit distinct, well-bounded distributions, enabling effective perception of degradation-related properties and facilitating the learning of a mapping relationship that bridges the degraded features and clear ones together. This conclusion has been confirmed in pre-trained VGG16, as shown in Fig. \ref{fig:gram}. In this section, a consistent phenomenon can be found in ResNet50, demonstrating the generality of our DCP. 

Specifically, similar to Section \ref{sec:dcp}, we firstly used the same three sets of 100 unpaired images as input, and utilized the “layer1” of ResNet50 as the feature extractor to extract different types of shallow features. After that, we leveraged the t-SNE to directly visualize the distributions of three sets of features, as shown in the gray dot area of Fig. \ref{fig:sup_gram}. It can be seen that, although there is a weak drift between features of different types, they are more mixed together, resulting in an indistinguishable cluster. 

Therefore, to tackle this issue, we computed the pairwise channel correlations for each set of features using Eq. \ref{form:gram}, resulting in three sets of channel correlation matrices, similar to the third column in Fig. \ref{fig:gram}. Finally, we visualized the distribution of the upper triangular part of these matrices with different types using t-SNE, represented by the colored points in Fig. \ref{fig:sup_gram}. It is clear that, the channel correlations of features with the same type have uniform distribution even if they have different content and semantics. Furthermore, when derived from different types of features, these correlations exhibit distinct margins according to corruption types. 
\begin{figure}[htbp]
\centering
\includegraphics[width=0.9\linewidth]{Figure/Visio-Fig8-Gram.pdf}
\caption{Deep Channel Prior is also verified in ResNet50.}
\label{fig:sup_gram}
\end{figure}

\section{Empirical Configurations within Method}
\label{sec:sup_config}
\textbf{Subsequent Two Layers for Multi-adversarial Mechanism.} As mentioned in Section \ref{section:stage1}, we empirically choose the subsequent two layers after enhancement as the equipment layers of multi-scale discriminators. For VGG16, we choose the “Conv1\_2” as the feature enhancement layer, and equip the discriminators on subsequent "Conv2\_1" and "Conv2\_2". For ResNet50, the "layer1" serves as the enhancement layer, accompanied by "layer2" and "layer3" as continuous discriminant layers. Similarly, for YOLOv5, we choose "C3\_1" as the enhancement layer and incorporate "C3\_2" and "C3\_3" as consecutive discrimination layers. As for DeepLabv3+, which leverages ResNet101 as the backbone, its configuration mirrors that of ResNet50.

\textbf{Layers for Correlation-consistent Loss in Various Backbones.} As illustrated in Section \ref{section:stage2}, we apply the correlation-consistent loss $L_{correlation}$ to the layers “Conv1\_2”, “Conv2\_2”, “Conv3\_3”, and “Conv4\_3” in VGG16. However,  the configuration of $L_{correlation}$ varies across different networks. In the case of ResNet50, we assess the correlation matrices in “layer1”, “layer2”, “layer3”, and “layer4”. For YOLOv5, we enforce consistency loss in “C3\_1”, “C3\_2”, “C3\_3”, and “C3\_4”. As for DeepLabv3+, leveraging ResNet101 as the backbone, its setup aligns with that of ResNet50.

\textbf{Empirical Weight Values for Each Loss Function.} For the multi-adversarial mechanism in Stage-1, we emphasize discrimination at the feature translation layer by assigning it a higher weight, while reducing the weights with increasing layers, specifically $w_1=0.5, w_2=0.3, w_3=0.2$. Regarding the diverse losses in Stage-1, we empirically set $\lambda_1=5, \lambda_2=10, \lambda_3=5$ for the adversarial loss $L_{adv}$, cycle-consistent loss $L_{cyc}$, and identity-preserving loss $L_{idt}$, respectively. Moving to the correlation-consistent loss in Stage-2, we argue that the feature correlations in deep layers better reflect their degradation types.  Therefore, we set $w_1=1, w_2=2, w_3=3, w_4=4$ based on empirical observations. Finally, for the diverse losses in Stage-2, we empirically set $\lambda_1=1000, \lambda_2=5, \lambda_3=10$ for the correlation-consistent loss $L_{correlation}$, adversarial loss $L_{adv}$, and content-consistent loss $L_{content}$, respectively.

\textbf{Detailed Structures of Generator Modules.} In our experiments, based on the varied demands for global and local information in various tasks, we designed two distinct generator structures, as illustrated in Fig. \ref{fig:sup_generator} (a) and (b). Specifically, a flattened structure with residual connections is consistently employed in low-quality image classification, while a U-Net structure composed of encoder-decoder is often utilized in foggy object detection and nighttime semantic segmentation. As for the structure of discriminators, we utilize PatchGAN for real/fake discrimination.
\begin{figure}[htbp]
\centering
\includegraphics[width=0.95\linewidth]{Figure/Visio-Fig9-Generator.pdf}
\caption{Different generator structures are used in various tasks.}
\label{fig:sup_generator}
\end{figure}

\section{More Implementation Details}
\label{sec:sup_impl}
\textbf{Datasets.} We conduct extensive experiments on eight benchmark datasets to evaluate the effectiveness of our UFEM, including one synthetic and 7 real-world datasets. Tab. \ref{tab:sup_datasets} provides a summary of crucial statistics for the employed datasets. 
\input{Table/Sup_Datasets}

\textbf{Detailed Settings for Each Comparison Method.} As mentioned above, we conduct comparisons on both synthetic and real datasets. Before conducting comparisons, it is noteworthy that, we fine-tuned the models to obtain well-performing classifiers, detectors, or segmenters on clear images. Taking fine-tuning for image classification on Haze-20 as an example, we initially selected 100 clear images per class from HazeClear-20 (80 for training, 20 for validation, and the remainder for testing) to fine-tune the pret-rained classifiers (VGG16 and ResNet50). After that, we obtained 20 classifiers that achieved accuracies of 95.9\% and 93.9\% on the test set, respectively. Next, we provide detailed descriptions of the settings for various comparison methods on these two types of datasets. 

On the synthetic dataset ImageNet-C, we mainly compared 15 kinds of IR (both supervised and unsupervised methods) and UDA methods. \textbf{For unsupervised image restoration methods}, \emph{e.g.}, D4, RefineDNet, EnGAN, and NeRCo, we randomly selected 1200 pairs of unpaired images from each degradation level for model training. After that, validation was performed on a test set of 50,000 images, synthesized based on \cite{hendrycks2019benchmarking}, derived from ImageNet. \textbf{For supervised image restoration}, \emph{e.g.}, C2PNet and CUE, we primarily utilized their officially released pre-trained weights for testing, which was consistent across real datasets. Besides, \textbf{for UDA methods} that require retraining models with unpaired but semantic-aligned images, we selected 10 pairs of unpaired images from each class of ImageNet and its degraded versions, forming a dataset of 10K images for retraining. However, since the settings of UDA methods are not applicable to the real world, we mainly compared our UFEM with the IR methods on real datasets.

On the real datasets, we focus on two authentic degradation scenarios: haze and low-light, along with three high-level visual tasks, including classification, detection, and segmentation. \textbf{For real hazy scenes}, to ensure fair comparisons, we randomly selected 500 unpaired images from the Haze-20 and its corresponding clear set, HazeClear-20, for training various UIR methods. These trained weights were then utilized for testing in the tasks of foggy image classification and foggy object detection. \textbf{For real low-light scenes}, similar to the above, we intended to create an unpaired dataset from the ExDARK. However, there is no corresponding clear version in this case. Therefore, following the collection in \cite{loh2019getting}, we manually selected images of the same categories as ExDARK from the ImageNet, PASCAL VOC, and COCO datasets, and filtered out the obviously low-light images, keeping only the clear images and ultimately obtained the clear dataset ExDARK-clean. After that, we randomly selected 500 unpaired images from ExDARK and ExDARK-clean for the training of UIR methods. These trained weights were then utilized for testing within dark image classification. However, \textbf{for nighttime semantic segmentation}, given their datasets' significantly higher resolution compared to ExDARK, we leveraged the pre-trained weights from IR methods for testing.

\section{More Quantitative and Qualitative Analysis}
\label{sec:sup_exp}
\subsection{More results for Image Classification} 
\textbf{Quantitative results on Motion Blur and Low Contrast.} In this part, we further compare our UFEM with 15 kinds of UIR and UDA methods on Motion Blur and Low Contrast from ImageNet-C. As reported in Tab. \ref{tab:blur_contrast}, our UFEM consistently outperforms the majority of UIR and UDA methods, demonstrating the competitiveness of our method across various degradation types and levels. Besides,

\begin{table*}[htbp]
    \centering
    \caption{The comparisons of our proposed UFEM with Unsupervised Image Restoration (UIR) and Unsupervised Domain Adaption (UDA) methods under three different degradation types, \emph{i.e.}, Motion Blur and Low Contrast. Each corruption type contains 5 severity levels.}
    \label{tab:blur_contrast}
    \resizebox{\textwidth}{!}{
    
    \begin{tabular}{lcccccccccccc}
    \Xhline{1.5pt}
                                  &                                  & \multicolumn{1}{c||}{}                                & \multicolumn{5}{c||}{\textbf{Top-1 Accuracy of VGG16 (\%)}}                                                                                                                                                                                                                                                                                 & \multicolumn{5}{c}{\textbf{Top-1 Accuracy of ResNet50 (\%)}}                                                                                                                                                                                                                                                        \\ \cline{4-13} 
\multirow{-2}{*}{\textbf{Method}} & \multirow{-2}{*}{\textbf{Venue}} & \multicolumn{1}{c||}{\multirow{-2}{*}{\textbf{Type}}} & \multicolumn{1}{c|}{\textbf{Level-1}}                           & \multicolumn{1}{c|}{\textbf{Level-2}}                           & \multicolumn{1}{c|}{\textbf{Level-3}}                            & \multicolumn{1}{c|}{\textbf{Level-4}}                            & \multicolumn{1}{c||}{\textbf{Level-5}}                           & \multicolumn{1}{c|}{\textbf{Level-1}}                           & \multicolumn{1}{c|}{\textbf{Level-2}}                           & \multicolumn{1}{c|}{\textbf{Level-3}}                           & \multicolumn{1}{c|}{\textbf{Level-4}}                           & \textbf{Level-5}                           \\ \hline

\multicolumn{13}{c}{\cellcolor[HTML]{EAEAEA}\textbf{Degradation Type: Motion Blur} (\textbf{100} unpaired images for UFEM, \textbf{1200} unpaired images for UIR methods, \textbf{10K} unpaired images for UDA methods)}                   \\ \hline
Baseline                 & -                  & \multicolumn{1}{c||}{\textbf{-}}                      & \multicolumn{1}{c|}{55.0}                                       & \multicolumn{1}{c|}{40.7}                                       & \multicolumn{1}{c|}{24.0}                                        & \multicolumn{1}{c|}{12.7}                                        & \multicolumn{1}{c||}{8.30}                                       & \multicolumn{1}{c|}{64.5}                                       & \multicolumn{1}{c|}{53.9}                                       & \multicolumn{1}{c|}{37.5}                                       & \multicolumn{1}{c|}{21.9}                                       & 14.8                                       \\
{CycleGAN}                 & {ICCV'17}                          & \multicolumn{1}{c||}{UIR}                    
 & \multicolumn{1}{c|}{46.5}        & \multicolumn{1}{c|}{36.2}         & \multicolumn{1}{c|}{23.1}         & \multicolumn{1}{c|}{14.2}         & \multicolumn{1}{c||}{\color[HTML]{3531ff}{\textbf{11.6 (3.3↑)}}}  & \multicolumn{1}{c|}{57.8}        & \multicolumn{1}{c|}{49.2}        & \multicolumn{1}{c|}{36.0}         & \multicolumn{1}{c|}{24.5}         & {\color[HTML]{3531ff}{\textbf{20.1 (5.3↑)}}}\\

UID-GAN                  & TBIOM'19                  & \multicolumn{1}{c||}{UIR}                    & \multicolumn{1}{c|}{39.0}                                       & \multicolumn{1}{c|}{22.3}                                       & \multicolumn{1}{c|}{8.10}                                        & \multicolumn{1}{c|}{3.60}                                        & \multicolumn{1}{c||}{2.30}                                       & \multicolumn{1}{c|}{50.1}                                       & \multicolumn{1}{c|}{33.5}                                       & \multicolumn{1}{c|}{13.6}                                       & \multicolumn{1}{c|}{5.90}                                       & 3.70                                       \\
DBGAN                    & CVPR'20                  & \multicolumn{1}{c||}{UIR}                    & \multicolumn{1}{c|}{{\color[HTML]{3531ff} \textbf{55.6 (0.6↑)}}}    & \multicolumn{1}{c|}{{\color[HTML]{3531ff} \textbf{44.7 (4.0↑)}}}    & \multicolumn{1}{c|}{{\color[HTML]{3531ff} \textbf{28.6 (4.6↑)}}}     & \multicolumn{1}{c|}{{\color[HTML]{3531ff} \textbf{15.4 (2.7↑)}}}     & \multicolumn{1}{c||}{\color[HTML]{000000} 10.0}                           & \multicolumn{1}{c|}{63.9}                                       & \multicolumn{1}{c|}{{\color[HTML]{3531ff} \textbf{56.8 (2.9↑)}}}    & \multicolumn{1}{c|}{{\color[HTML]{3531ff} \textbf{42.4 (4.9↑)}}}    & \multicolumn{1}{c|}{{\color[HTML]{3531ff} \textbf{25.3 (3.4↑)}}} & 17.1                                       \\
FCL-GAN                  & ACM MM'22                  & \multicolumn{1}{c||}{UIR}                    & \multicolumn{1}{c|}{54.5}                                       & \multicolumn{1}{c|}{42.2}                                       & \multicolumn{1}{c|}{25.7}                                        & \multicolumn{1}{c|}{13.5}                                        & \multicolumn{1}{c||}{5.70}                                       & \multicolumn{1}{c|}{{\color[HTML]{3531ff} \textbf{64.9 (0.4↑)}}}    & \multicolumn{1}{c|}{55.7}                                       & \multicolumn{1}{c|}{40.7}                                       & \multicolumn{1}{c|}{24.9}                                       & 13.1                                       \\
CRNet                    & ACM MM'22                  & \multicolumn{1}{c||}{UIR}                    & \multicolumn{1}{c|}{22.9}                                       & \multicolumn{1}{c|}{17.6}                                       & \multicolumn{1}{c|}{6.40}                                        & \multicolumn{1}{c|}{2.90}                                        & \multicolumn{1}{c||}{3.90}                                       & \multicolumn{1}{c|}{32.7}                                       & \multicolumn{1}{c|}{27.2}                                       & \multicolumn{1}{c|}{11.9}                                       & \multicolumn{1}{c|}{5.70}                                       & 6.60                                       \\ 
DAN                     & PMLR'15                  & \multicolumn{1}{c||}{UDA}                    & \multicolumn{1}{c|}{29.0}         & \multicolumn{1}{c|}{17.4}         & \multicolumn{1}{c|}{8.80}          & \multicolumn{1}{c|}{4.80}          & \multicolumn{1}{c||}{3.30}          & \multicolumn{1}{c|}{48.6}        & \multicolumn{1}{c|}{30.4}        & \multicolumn{1}{c|}{33.5}         & \multicolumn{1}{c|}{22.2}         & 11.6     \\

MDD                     & PMLR'19                  & \multicolumn{1}{c||}{UDA}                     & \multicolumn{1}{c|}{24.7}         & \multicolumn{1}{c|}{16.6}         & \multicolumn{1}{c|}{9.50}          & \multicolumn{1}{c|}{5.00}   & \multicolumn{1}{c||}{3.90}   & \multicolumn{1}{c|}{54.9}        & \multicolumn{1}{c|}{38.8}        & \multicolumn{1}{c|}{22.6}         & \multicolumn{1}{c|}{19.9}         & 14.6             \\

CGDM                     & CVPR'21                  & \multicolumn{1}{c||}{UDA}                    & \multicolumn{1}{c|}{{\color[HTML]{000000} 39.7}}                & \multicolumn{1}{c|}{{\color[HTML]{000000} 28.6}}                & \multicolumn{1}{c|}{{\color[HTML]{000000} 14.8}}                 & \multicolumn{1}{c|}{3.00}                                        & \multicolumn{1}{c||}{1.80}                                       & \multicolumn{1}{c|}{{\color[HTML]{000000} 60.3}}                & \multicolumn{1}{c|}{{\color[HTML]{000000} 52.9}}                & \multicolumn{1}{c|}{{\color[HTML]{000000} 40.8}}                & \multicolumn{1}{c|}{{\color[HTML]{000000} 24.7}}    & {\color[HTML]{000000} 19.2}    \\ 

DAN-TransPar             & TIP'22                  & \multicolumn{1}{c||}{UDA}                    & \multicolumn{1}{c|}{29.1}                                       & \multicolumn{1}{c|}{17.2}                                       & \multicolumn{1}{c|}{8.60}                                        & \multicolumn{1}{c|}{4.50}                                        & \multicolumn{1}{c||}{3.30}                                       & \multicolumn{1}{c|}{44.6}                                       & \multicolumn{1}{c|}{30.1}                                       & \multicolumn{1}{c|}{0.10}                                       & \multicolumn{1}{c|}{0.70}                                       & 9.30                                       \\
MDD-TransPar             & TIP'22                  & \multicolumn{1}{c||}{UDA}                    & \multicolumn{1}{c|}{29.0}                                       & \multicolumn{1}{c|}{13.6}                                       & \multicolumn{1}{c|}{8.10}                                        & \multicolumn{1}{c|}{4.20}                                        & \multicolumn{1}{c||}{3.10}                                       & \multicolumn{1}{c|}{56.7}                                       & \multicolumn{1}{c|}{42.9}                                       & \multicolumn{1}{c|}{26.8}                                       & \multicolumn{1}{c|}{16.3}                                       & 12.0                                       \\

\hline
\textbf{UFEM (Ours)}                & \textbf{-}                  & \multicolumn{1}{c||}{\textbf{-}}                    & \multicolumn{1}{c|}{{\color[HTML]{fe0000} \textbf{59.7 (4.7↑)}}} & \multicolumn{1}{c|}{{\color[HTML]{fe0000} \textbf{50.6 (9.9↑)}}} & \multicolumn{1}{c|}{{\color[HTML]{fe0000} \textbf{34.7 (10.7↑)}}} & \multicolumn{1}{c|}{{\color[HTML]{fe0000} \textbf{22.8 (10.1↑)}}} & \multicolumn{1}{c||}{{\color[HTML]{fe0000} \textbf{15.3 (7.0↑)}}} & \multicolumn{1}{c|}{{\color[HTML]{fe0000} \textbf{65.7 (1.3↑)}}} & \multicolumn{1}{c|}{{\color[HTML]{fe0000} \textbf{58.2 (4.3↑)}}} & \multicolumn{1}{c|}{{\color[HTML]{fe0000} \textbf{43.1 (5.6↑)}}} & \multicolumn{1}{c|}{{\color[HTML]{fe0000} \textbf{26.7 (4.8↑)}}}                & {\color[HTML]{fe0000} \textbf{20.1 (5.3↑)}}   \\ \hline

\multicolumn{13}{c}{\cellcolor[HTML]{EAEAEA}\textbf{Degradation Type: Low Contrast} (\textbf{100} unpaired images for UFEM, \textbf{1200} unpaired images for UIR methods, \textbf{10K} unpaired images for UDA methods)}              \\ \hline
Baseline                 & -                  & \multicolumn{1}{c||}{\textbf{-}}                      & \multicolumn{1}{c|}{56.9}                                       & \multicolumn{1}{c|}{48.2}                                       & \multicolumn{1}{c|}{32.3}                                        & \multicolumn{1}{c|}{10.3}                                        & \multicolumn{1}{c||}{2.50}                                       & \multicolumn{1}{c|}{64.3}                                       & \multicolumn{1}{c|}{57.8}                                       & \multicolumn{1}{c|}{45.5}                                       & \multicolumn{1}{c|}{20.3}                                       & 5.40                                       \\
{CycleGAN}                 & {ICCV'17}                          & \multicolumn{1}{c||}{UIR}                    
& \multicolumn{1}{c|}{54.6}        & \multicolumn{1}{c|}{51.1}         & \multicolumn{1}{c|}{\color[HTML]{3531ff}{\textbf{47.0 (14.7↑)}}} & \multicolumn{1}{c|}{\color[HTML]{3531ff}{\textbf{31.9 (21.6↑)}}} & \multicolumn{1}{c||}{\color[HTML]{3531ff}{\textbf{12.4 (9.9↑)}}}  & \multicolumn{1}{c|}{63.4}        & \multicolumn{1}{c|}{60.5}        & \multicolumn{1}{c|}{\textcolor[RGB]{255,0,0}{\textbf{57.3 (11.8↑)}}} & \multicolumn{1}{c|}{\textcolor[RGB]{255,0,0}{\textbf{43.6 (23.3↑)}}} & \textcolor[RGB]{255,0,0}{\textbf{20.8 (15.4↑)}}                                      
\\
EnligntenGAN             & TIP'21                  & \multicolumn{1}{c||}{UIR}                    & \multicolumn{1}{c|}{\color[HTML]{3531ff} \textbf{58.7 (1.8↑)}}                           & \multicolumn{1}{c|}{\color[HTML]{3531ff} \textbf{52.5 (4.3↑)}}                           & \multicolumn{1}{c|}{\color[HTML]{000000} 34.8}                            & \multicolumn{1}{c|}{\color[HTML]{000000} 11.4}                            & \multicolumn{1}{c||}{\color[HTML]{000000} 2.70}                           & \multicolumn{1}{c|}{\color[HTML]{fe0000} \textbf{66.0 (1.7↑)}}                        & \multicolumn{1}{c|}{\color[HTML]{3531ff} \textbf{60.7 (2.9↑)}}                           & \multicolumn{1}{c|}{47.3}                                       & \multicolumn{1}{c|}{22.3}                                       & 6.70                                       \\
Zero-DCE                 & CVPR'20                  & \multicolumn{1}{c||}{UIR}                    & \multicolumn{1}{c|}{21.1}                                       & \multicolumn{1}{c|}{11.3}                                       & \multicolumn{1}{c|}{6.50}                                        & \multicolumn{1}{c|}{1.50}                                        & \multicolumn{1}{c||}{0.50}                                       & \multicolumn{1}{c|}{27.7}                                       & \multicolumn{1}{c|}{16.0}                                       & \multicolumn{1}{c|}{9.00}                                       & \multicolumn{1}{c|}{1.90}                                       & 0.50                                       \\
ZeroDCE++                & TPAMI'21                  & \multicolumn{1}{c||}{UIR}                    & \multicolumn{1}{c|}{45.8}                                       & \multicolumn{1}{c|}{36.2}                                       & \multicolumn{1}{c|}{19.7}                                        & \multicolumn{1}{c|}{5.70}                                        & \multicolumn{1}{c||}{1.50}                                       & \multicolumn{1}{c|}{56.0}                                       & \multicolumn{1}{c|}{48.1}                                       & \multicolumn{1}{c|}{31.7}                                       & \multicolumn{1}{c|}{11.3}                                       & 2.70                                       \\
LE-GAN                   & KBS'22                  & \multicolumn{1}{c||}{UIR}                    & \multicolumn{1}{c|}{52.1}                                       & \multicolumn{1}{c|}{47.2}                                       & \multicolumn{1}{c|}{5.40}                                        & \multicolumn{1}{c|}{1.70}                                        & \multicolumn{1}{c||}{0.30}                                       & \multicolumn{1}{c|}{60.3}                                       & \multicolumn{1}{c|}{56.3}                                       & \multicolumn{1}{c|}{8.40}                                       & \multicolumn{1}{c|}{2.80}                                       & 0.50                                       \\ 
DAN                     & PMLR'15                  & \multicolumn{1}{c||}{UDA}                    & \multicolumn{1}{c|}{23.8}         & \multicolumn{1}{c|}{17.5}         & \multicolumn{1}{c|}{11.0}         & \multicolumn{1}{c|}{3.50}          & \multicolumn{1}{c||}{1.00}          & \multicolumn{1}{c|}{53.3}        & \multicolumn{1}{c|}{35.9}        & \multicolumn{1}{c|}{43.6}         & \multicolumn{1}{c|}{23.7}         & 6.70                        \\ 
MDD                     & PMLR'19                  & \multicolumn{1}{c||}{UDA}                    & \multicolumn{1}{c|}{21.9}         & \multicolumn{1}{c|}{13.3}         & \multicolumn{1}{c|}{8.50}          & \multicolumn{1}{c|}{3.80}          & \multicolumn{1}{c||}{1.50}          & \multicolumn{1}{c|}{53.7}        & \multicolumn{1}{c|}{45.3}        & \multicolumn{1}{c|}{31.3}         & \multicolumn{1}{c|}{20.9}         & 8.20                        \\ 
CGDM                     & CVPR'21                  & \multicolumn{1}{c||}{UDA}                    & \multicolumn{1}{c|}{44.5}                                       & \multicolumn{1}{c|}{40.4}                                       & \multicolumn{1}{c|}{33.3}                                        & \multicolumn{1}{c|}{7.80}                                        & \multicolumn{1}{c||}{1.70}                                       & \multicolumn{1}{c|}{61.6}                                       & \multicolumn{1}{c|}{58.5}                                       & \multicolumn{1}{c|}{\color[HTML]{3531ff} \textbf{53.4 (7.9↑)}}                        & \multicolumn{1}{c|}{\color[HTML]{3531ff} \textbf{34.3 (14.0↑)}}                       & \color[HTML]{3531ff} \textbf{12.0 (6.6↑)}                        \\ 

DAN-TransPar             & TIP'22                  & \multicolumn{1}{c||}{UDA}                    & \multicolumn{1}{c|}{23.4}                                       & \multicolumn{1}{c|}{17.7}                                       & \multicolumn{1}{c|}{10.4}                                        & \multicolumn{1}{c|}{3.20}                                        & \multicolumn{1}{c||}{1.10}                                       & \multicolumn{1}{c|}{45.6}                                       & \multicolumn{1}{c|}{48.0}                                       & \multicolumn{1}{c|}{11.9}                                       & \multicolumn{1}{c|}{0.10}                                       & 5.40                                       \\
MDD-TransPar             & TIP22                  & \multicolumn{1}{c||}{UDA}                    & \multicolumn{1}{c|}{19.1}                                       & \multicolumn{1}{c|}{11.6}                                       & \multicolumn{1}{c|}{7.40}                                        & \multicolumn{1}{c|}{3.20}                                        & \multicolumn{1}{c||}{1.30}                                       & \multicolumn{1}{c|}{57.0}                                       & \multicolumn{1}{c|}{41.7}                                       & \multicolumn{1}{c|}{26.2}                                       & \multicolumn{1}{c|}{15.8}                                       & 5.70                                       \\

\hline
\textbf{UFEM (Ours)}                & \textbf{-}                  & \multicolumn{1}{c||}{\textbf{-}}                    & \multicolumn{1}{c|}{\color[HTML]{fe0000} \textbf{62.8 (5.9↑)}}                        & \multicolumn{1}{c|}{\color[HTML]{fe0000} \textbf{58.8 (10.6↑)}}                       & \multicolumn{1}{c|}{\color[HTML]{fe0000} \textbf{53.0 (20.7↑)}}                        & \multicolumn{1}{c|}{\color[HTML]{fe0000} \textbf{32.0 (21.7↑)}}                        & \multicolumn{1}{c||}{\color[HTML]{fe0000} \textbf{14.5 (12.0↑)}}                       & \multicolumn{1}{c|}{\color[HTML]{3531ff} \textbf{65.0 (0.7↑)}}                           & \multicolumn{1}{c|}{\color[HTML]{fe0000} \textbf{60.8 (3.0↑)}}                        & \multicolumn{1}{c|}{\color[HTML]{000000} 48.5}                           & \multicolumn{1}{c|}{\color[HTML]{000000} 23.2}                           & {\color[HTML]{000000} 8.40}          \\ \Xhline{1.5pt}
\end{tabular}
}
\end{table*}

\textbf{Grad-CAM Attention Comparison with IR methods.}

\textbf{Visual Analysis of T-SNE Dimensionality Reduction.}

\subsection{More results for Object Detection}
\textbf{Grad-CAM Attention Comparison with IR methods.}

\subsection{More results for Semantic Segmentation}
\textbf{Comparison of segmentation results with IR methods.}
